# Supplementary material for: Prediction of the onset of cardiovascular diseases from electronic health records using multi-task gated recurrent units
Source: arXiv:2007.08491 ancillary file (2020-07-16)
Supplement: Supplementary file 1 [file Supplementary_Material.pdf]

Supplementary Material: Prediction of the onset of  
cardiovascular diseases from electronic health records using  
multi-task gated recurrent units

Fernando Andreotti, Frank S. Heldt, Basel Abu-Jamous, Ming Li,  
Avelino Javier, Oliver Carr, Stojan Jovanovic,  
Nadezda Lipunova, Benjamin Irving, Rabia T. Khan, Robert Dürichen

July 14, 2020

# 1 MT attention GRU (MT-Att-GRU) model and hyperparameter tuning

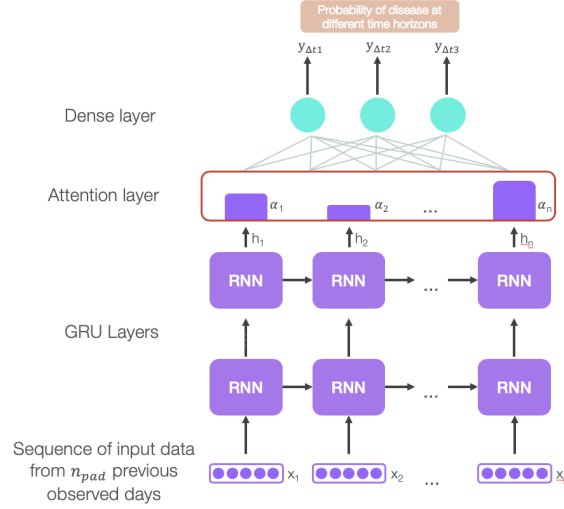

Figure 1: Representation of MT-Att-GRU model.

The proposed model receives a padded sequence of  $n_{pad}$  observation days and  $n_{features}$  for each sample patient  $P$ . The underlying model contains  $n_L$  gated recurrent unit (GRU) network recurrent layers each with  $n_{units}$  hidden units, on top of which we use Luong’s attention mechanism [LPM15] assigns weights to each observed timestep (i.e. day). Lastly, a fully connected layer with sigmoid activation and  $n_{out} = 4$  nodes, one for each time horizon (i.e. 1, 3, 12 and  $> 12$  months), was used. Within each GRU layer a recurrent L2 regularisation was applied with weight  $l_2$  and recurrent activation  $\sigma_g$ . Layer normalisation was used after each recurrent activation, followed by a dropout layer with probability  $p_{drop}$ . Were trained with the *adam* optimizer with learning rate  $l_r$ , early stopping (penalty of 10 epochs without improvement) and binary cross entropy as loss function.

All GRU-based models were optimized using a Bayesian optimisation scheme. Optimisation parameters are described in Table 1. Search used 50 iterations and 20 epochs. The final model then was evaluated on a 5-fold cross-validation procedure with 100 epochs for training.

Table 1: Hyperparameters of the proposed neural network searched using Bayesian optimisation.

| Hyperparameter | Brief Description                              | Search Range   |
|----------------|------------------------------------------------|----------------|
| $n_{pad}$      | Number of observed days for padding            | [1, 100]       |
| $n_L$          | Number of recurrent layers                     | {1, 2, 3}      |
| $n_{units}$    | Number of hidden units in each recurrent layer | [16, 128]      |
| $n_{pad}$      | Number of observation days for padding         | [10, 100]      |
| $p_{drop}$     | Dropout rate                                   | [0, 0.5]       |
| $l_r$          | Learning Rate                                  | $[10^4, 10^2]$ |
| $l_2$          | L2 regularisation                              | $[10^4, 10^1]$ |

## 2 Additional Results

The results for logistic regression (LR) classification using different number of past observation days are presented in Table 2.

Table 2: Performances of Logistic Regression variants in predicting myocardial infarction and ischemic stroke throughout all time horizons. Shown are average and standard deviation of area under the curve (AUC), sensitivity (Sen), and precision (Prec) of 5-fold cross validation. Best average results per time horizon and disease are highlighted in bold.

| Time horizon | Method  | Myocardial Infarction |                   |                   | Stroke            |                   |                   |
|--------------|---------|-----------------------|-------------------|-------------------|-------------------|-------------------|-------------------|
|              |         | AUC                   | Sen               | Prec              | AUC               | Sen               | Prec              |
| 1 month      | MT GRU  | 0.763 $\pm$ 0.032     | 0.694 $\pm$ 0.124 | 0.138 $\pm$ 0.016 | 0.722 $\pm$ 0.014 | 0.608 $\pm$ 0.087 | 0.188 $\pm$ 0.035 |
|              | LR(1)   | 0.702 $\pm$ 0.054     | 0.772 $\pm$ 0.136 | 0.657 $\pm$ 0.062 | 0.694 $\pm$ 0.036 | 0.649 $\pm$ 0.143 | 0.687 $\pm$ 0.069 |
|              | LR(50)  | 0.702 $\pm$ 0.054     | 0.772 $\pm$ 0.136 | 0.657 $\pm$ 0.062 | 0.597 $\pm$ 0.028 | 0.546 $\pm$ 0.134 | 0.631 $\pm$ 0.020 |
|              | LR(100) | 0.599 $\pm$ 0.034     | 0.650 $\pm$ 0.161 | 0.589 $\pm$ 0.014 | 0.695 $\pm$ 0.039 | 0.649 $\pm$ 0.143 | 0.69 $\pm$ 0.072  |
| 3 months     | MT GRU  | 0.773 $\pm$ 0.010     | 0.707 $\pm$ 0.061 | 0.355 $\pm$ 0.043 | 0.734 $\pm$ 0.025 | 0.698 $\pm$ 0.069 | 0.371 $\pm$ 0.018 |
|              | LR(1)   | 0.740 $\pm$ 0.024     | 0.678 $\pm$ 0.094 | 0.693 $\pm$ 0.020 | 0.719 $\pm$ 0.015 | 0.712 $\pm$ 0.036 | 0.667 $\pm$ 0.025 |
|              | LR(50)  | 0.740 $\pm$ 0.024     | 0.678 $\pm$ 0.094 | 0.693 $\pm$ 0.020 | 0.679 $\pm$ 0.032 | 0.699 $\pm$ 0.092 | 0.641 $\pm$ 0.034 |
|              | LR(100) | 0.715 $\pm$ 0.010     | 0.689 $\pm$ 0.075 | 0.677 $\pm$ 0.017 | 0.720 $\pm$ 0.015 | 0.720 $\pm$ 0.028 | 0.664 $\pm$ 0.026 |
| 12 months    | MT GRU  | 0.811 $\pm$ 0.018     | 0.794 $\pm$ 0.045 | 0.594 $\pm$ 0.041 | 0.801 $\pm$ 0.010 | 0.765 $\pm$ 0.065 | 0.637 $\pm$ 0.033 |
|              | LR(1)   | 0.758 $\pm$ 0.005     | 0.660 $\pm$ 0.034 | 0.714 $\pm$ 0.014 | 0.751 $\pm$ 0.010 | 0.747 $\pm$ 0.086 | 0.681 $\pm$ 0.025 |
|              | LR(50)  | 0.758 $\pm$ 0.005     | 0.660 $\pm$ 0.034 | 0.714 $\pm$ 0.014 | 0.737 $\pm$ 0.018 | 0.691 $\pm$ 0.064 | 0.692 $\pm$ 0.034 |
|              | LR(100) | 0.772 $\pm$ 0.018     | 0.715 $\pm$ 0.053 | 0.724 $\pm$ 0.008 | 0.751 $\pm$ 0.010 | 0.729 $\pm$ 0.099 | 0.692 $\pm$ 0.032 |
| > 12 months  | MT GRU  | 0.897 $\pm$ 0.015     | 0.779 $\pm$ 0.023 | 0.847 $\pm$ 0.027 | 0.849 $\pm$ 0.009 | 0.774 $\pm$ 0.030 | 0.768 $\pm$ 0.018 |
|              | LR(1)   | 0.785 $\pm$ 0.008     | 0.706 $\pm$ 0.026 | 0.717 $\pm$ 0.020 | 0.767 $\pm$ 0.011 | 0.715 $\pm$ 0.022 | 0.700 $\pm$ 0.013 |
|              | LR(50)  | 0.785 $\pm$ 0.008     | 0.706 $\pm$ 0.026 | 0.717 $\pm$ 0.020 | 0.785 $\pm$ 0.017 | 0.686 $\pm$ 0.055 | 0.745 $\pm$ 0.017 |
|              | LR(100) | 0.819 $\pm$ 0.014     | 0.749 $\pm$ 0.040 | 0.767 $\pm$ 0.026 | 0.768 $\pm$ 0.010 | 0.724 $\pm$ 0.030 | 0.699 $\pm$ 0.012 |

### 2.1 Area under the curve plots for different time horizons

Receiver operating characteristic (ROC) curves for all time horizons are shown for both myocardial infarction (MI) and stroke cohorts on Fig. 2 and Fig. 3.

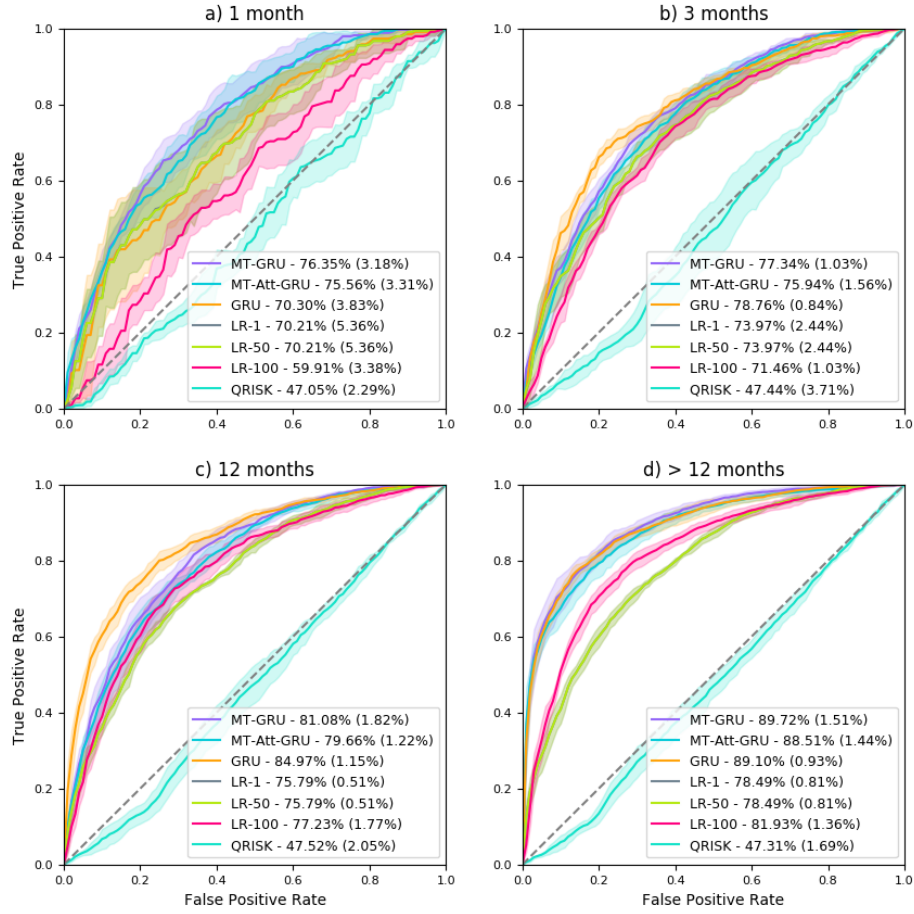

Figure 2: MI cohort average ROC and standard deviation brackets for the proposed models in comparison to LR with either 1, 50, or 100 number of observation days and QRISK to predict the risk of having myocardial infarction. Predicted time horizons shown (a) 1, (b) 3, (c) 12, and (d) > 12 months. Shaded areas represent the standard deviation based on 5-fold cross-validation.

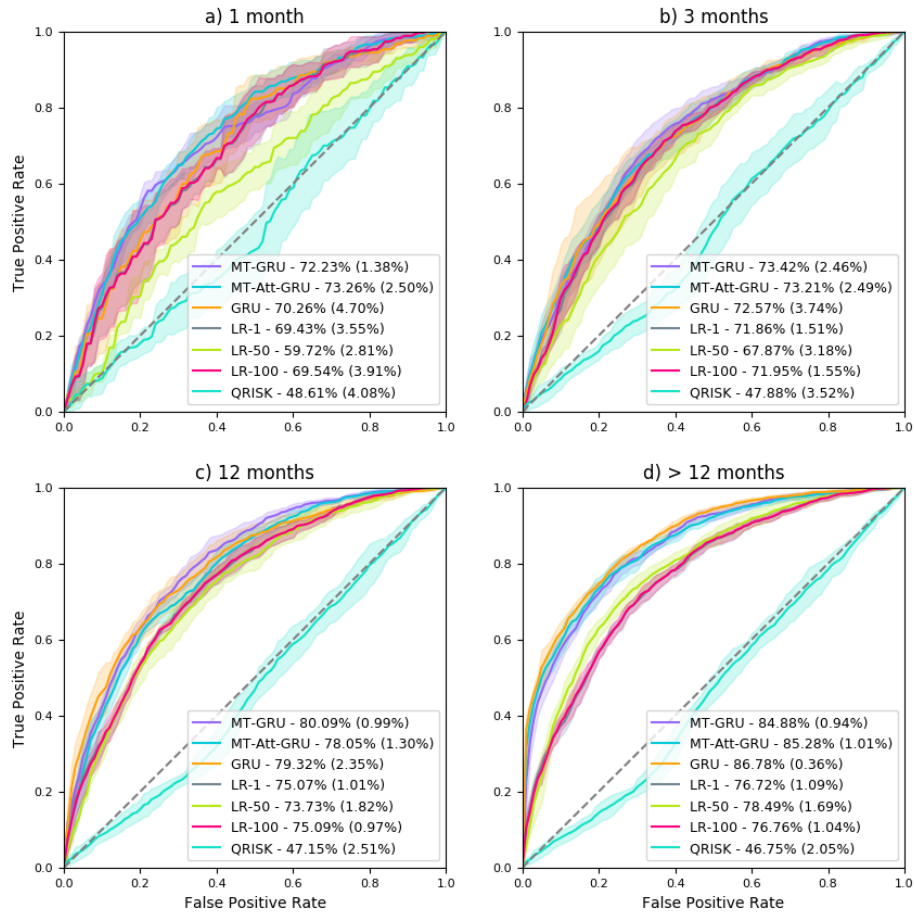

Figure 3: Ischaemic stroke cohort average ROC and standard deviation brackets for the proposed models in comparison to LR with either 1, 50, or 100 number of observation days and QRISK to predict the risk of having stroke. Predicted time horizons shown (a) 1, (b) 3, (c) 12, and (d) > 12 months. Shaded areas represent the standard deviation based on 5-fold cross-validation.

## 2.2 Feature Importance

Permutation feature importance for both cohorts presented in Fig. 4.

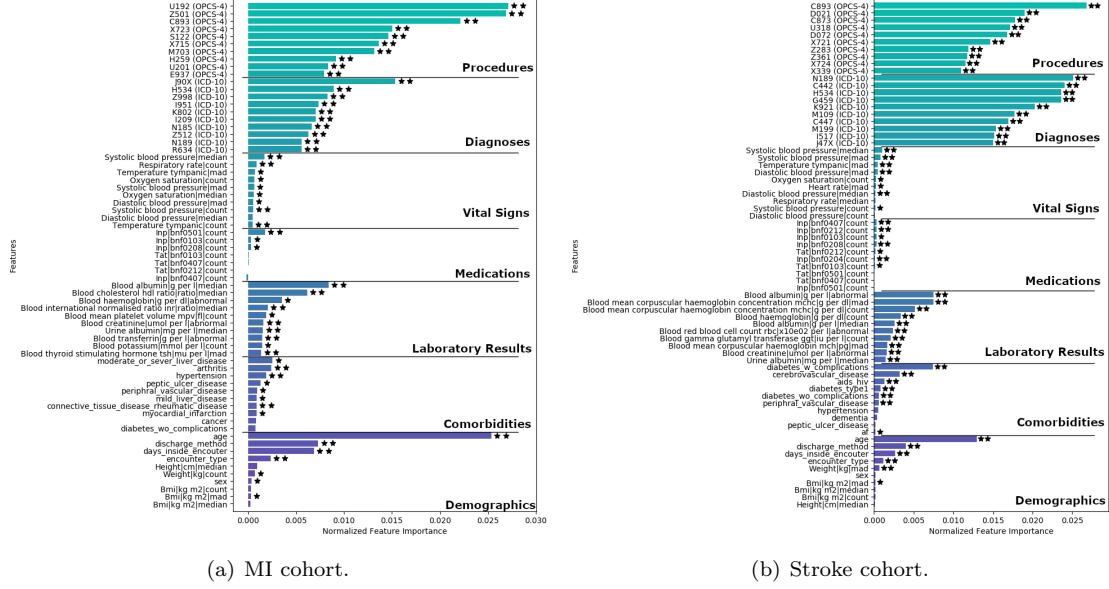

Figure 4: Comparison of feature importance across (a) MI and (b) stroke. Figures show results of MT GRU approach with a  $> 12$  months time horizon. In (a) asterisks mark significance from zero with t-test p-value thresholds of 5% (\*) and 1% (\*\*). At most, the top 10 features for each category is shown.

## Whole bibliography

[LPM15] Thang Luong, Hieu Pham, and Christopher D. Manning. “Effective Approaches to Attention-based Neural Machine Translation”. In: *Proceedings of the 2015 Conference on Empirical Methods in Natural Language Processing*. Stroudsburg, PA, USA, 2015, pp. 1412–1421.
